# Supplementary material for: Loschmidt echo approach to Krylov-subspace approximation error estimation
Source: arXiv:2107.09805 source file (2021-07-20)
Supplement: Supplementary file 1 [file appendix1.tex]

\section{\\Toeplitz} \label{sec:appendix}

A tridiagonal Toeplitz matrix is the particular case of the tridiagonal matrix with homogeneous coefficients $\alpha_k = \alpha$ and $\beta_k = \beta$ $\forall k$.

\begin{equation}
    \begin{pmatrix}\alpha & \beta & 0 & \cdots & 0\\
\beta & \alpha & \beta & \cdots & 0\\
0 & \beta & \alpha & \cdots & 0\\
\vdots & \vdots & \vdots & \ddots & \vdots\\
0 & 0 & 0 & \cdots & \alpha

\end{pmatrix}
\end{equation}

$\ket{\psi\left(t_0\right)}$

$\ket{\psi\left(t\right)}$

$\ket{\varphi_k\left(t\right)}$

$\braket{\varphi_k\left(t\right) | \psi\left(t\right)}$

$\braket{\varphi_k\left(t\right) | \varphi_{k,k+1}\left(t\right)}$

$e_{k} = ||\psi(t) - \psi_{k}(t)||$

$e_{k,k+1} \sim ||\psi_{k+1}(t) - \psi_{k}(t)||$

$\psi_{k+1}(t) = \psi(t) + \Delta\psi_{k+1}(t)$ 

$e_{k,k+1} = ||(\psi(t)- \psi_{k}(t)) + \Delta\psi_{k+1}(t) || <= ||(\psi(t)- \psi_{k}(t))|| + ||\Delta\psi_{k+1}(t)||$

$||(\psi(t)- \psi_{k}(t))|| - ||\Delta\psi_{k+1}(t)|| <= e_{k,k+1} <= ||(\psi(t)- \psi_{k}(t))|| + ||\Delta\psi_{k+1}(t)||$

\begin{equation*}
e_{k,k+1} - ||\Delta\psi_{k+1}(t)|| < ||(\psi(t)- \psi_{k}(t))|| < e_{k,k+1} + ||\Delta\psi_{k+1}(t)||
\end{equation*}

\begin{equation*}
e_{k,k+1} - e_{k+1} < e_{k} < e_{k,k+1} + e_{k+1}
\end{equation*}

Suponemos que es verdad la relacion lineal entre los errores

\begin{equation*}
e_{k,k+1}(t) - (a e_{k}(t) + b) < e_{k}(t) < e_{k,k+1}(t) + (a e_{k}(t) + b)
\end{equation*}

\begin{equation*}
\frac{e_{k,k+1}(t) - b}{1+a}< e_{k}(t) < \frac{{e_{k,k+1}(t)+ b}}{1-a}
\end{equation*}

\begin{equation*}
e_{k}(t) \sim e^{(-t^\alpha * k )}
\end{equation*}

\begin{equation}
e_{k+1}(t) = a e_{k}(t) + b
\end{equation}

\begin{equation}
    \psi(t) = \sum_{n=1}^{k} S_{1,n}^{k}(t) \psi_n
\end{equation}

\begin{equation}
    \psi(t) = \sum_{n=1}^{N} S_{1,n}^{N}(t) \psi_n
\end{equation}

\begin{equation}
    | S_{1,n}^{k}(t) - S_{1,n}^{N}(t)| \sim | S_{1,n}^{k}(t) - S_{1,n}^{k+1}(t)|
\end{equation}

\begin{equation}
     S_{1,n}^{k}(t) = \int_{c \in [0,k]} p(c)    
\end{equation}

\begin{equation}
     S_{1,n}^{N}(t) = \int_{c \in [0,N]} p(c)    
\end{equation}

\begin{equation}
     S_{1,n}^{k}(t) - S_{1,n}^{N}(t) = \int_{c \in [0,N] c>k} p(c)    
\end{equation}

\begin{equation}
     S_{1,n}^{k}(t) - S_{1,n}^{k+1}(t) = \int_{c \in [0,k+1] c>k} p(c) 
\end{equation}    

\begin{equation}
     S_{1,n}^{k}(t) - S_{1,n}^{N}(t) = \int_{c \in [0,N] c>k+1} p(c)
     + \int_{c \in [0,k+1] c>k} p(c)    
\end{equation}

$\sum_{n=1}^k S^{n}_{1\ \rightarrow n}(t) S^{N}_{n\ \rightarrow 1}(-t)$

\begin{equation}\label{eq:c6}
S^{n}_{1 \rightarrow n}(t) S^{N}_{n \rightarrow 1}(-t) = \sum_{p=1}^{N}\sum_{q=1}^{k}
\sin{\Big( \frac{\pi p}{N+1}\Big)}\sin{\Big( \frac{\pi p n}{N+1}\Big)}
\sin{\Big( \frac{\pi q}{k+1}\Big)}\sin{\Big( \frac{\pi q n}{k+1}\Big)}
e^{2it\beta \cos{\big( \frac{\pi p}{N+1} \big)} - \cos{\big( \frac{\pi q}{k+1} \big)} }
\end{equation}
